# Supplementary material for: Coherent shear wave in crystalline Si upon sub-threshold femtosecond laser-induced excitation
Source: arXiv:2503.10420 source file (2026-11-18)
Supplement: Supplementary file 1 [file anc_SM_MID_2024_UDD_SW.pdf]

# Supplementary Information: Imaging Ultrafast Dynamical Diffraction wavefronts of femtosecond laser-induced lattice distortions inside crystalline semiconductors

Angel Rodríguez-Fernández,* Jan-Etienne Pudell, Roman Shayduk, Wonhyuk Jo, James Wrigley, Johannes Möller, Peter Zalden, Alexey Zozulya, Jörg Hallmann, and Anders Madsen

*European XFEL Facility GmbH, Holzkoppel 4,Schenefeld DE, 22869*

Pablo Villanueva-Perez

*Division of Synchrotron Radiation Research and NanoLund, Department of Physics, Lund University, Lund, 22100 Sweden*

Zdenek Matej

*MAX IV Laboratory, Lund University, Lund, Sweden SE-22100*

Thies J. Albert, Dominik Kaczmarek, and Klaus Sokolowski-Tinten

*Department of Physics, Universitt Duisburg-Essen, Lotharstr. 1, 47057 Duisburg, Germany. and Center for Nanointegration Duisburg-Essen, Universität Duisburg-Essen, Carl-Benz-Str. 199, 47057 Duisburg, Germany*

Antonowicz Jerzy

*Faculty of Physics, Warsaw University of Technology, Koszykowa 75, 00-662 Warsaw, Poland*

Ryszard Sobierajski, Rahimi Mosafer, and Oleksii I. Liubchenko

*Institute of Physics of the Polish Academy of Sciences, Aleja Lotnikw 32/46, PL-02668 Warsaw, Poland*

Javier Solis and Jan Siegel†

*Laser Processing Group, Instituto de Optica (IO-CSIC), Consejo Superior de Investigaciones Científicas, CSIC, 28006, Madrid, Spain*

(Dated: April 3, 2025)


## Abstract

Material processing with femtosecond lasers has attracted enormous attention because of its potential for technology and industrial applications. In parallel, time-resolved x-ray diffraction has been successfully used to study ultrafast structural distortion dynamics in semiconductor thin films or surface layers of bulk materials. However, 'real-world' processing applications deal mostly with bulk materials, which prevents the use of such techniques. For processing applications, a fast and depth-sensitive probe is needed. To address this, we present a novel technique based on ultrafast dynamical diffraction (UDD) capable of imaging transient strain distributions inside bulk crystals upon single-pulse excitation. This pump-probe technique provides a complete picture of the temporal evolution of ultrafast distortion depth profiles. Our measurements were obtained in a thin crystalline Si wafer upon single pulse femtosecond optical excitation revealing that below the melting threshold strong lattice distortions appear on ps time scales due to the formation and propagation of strain waves into the bulk.


Keywords: Imaging, Ultrafast, Crystal Distortions, Laser, Dynamical Diffraction, XFEL

---

[1] C. Thomsen, H. T. Grahn, H. J. Maris, and J. Tauc, Surface generation and detection of phonons by picosecond light pulses, Phys. Rev. B **34**, 4129 (1986).

* Contact author: angel.rodriguez-fernandez@xfel.eu

† Contact author: j.siegel@io.cfmac.csic.es

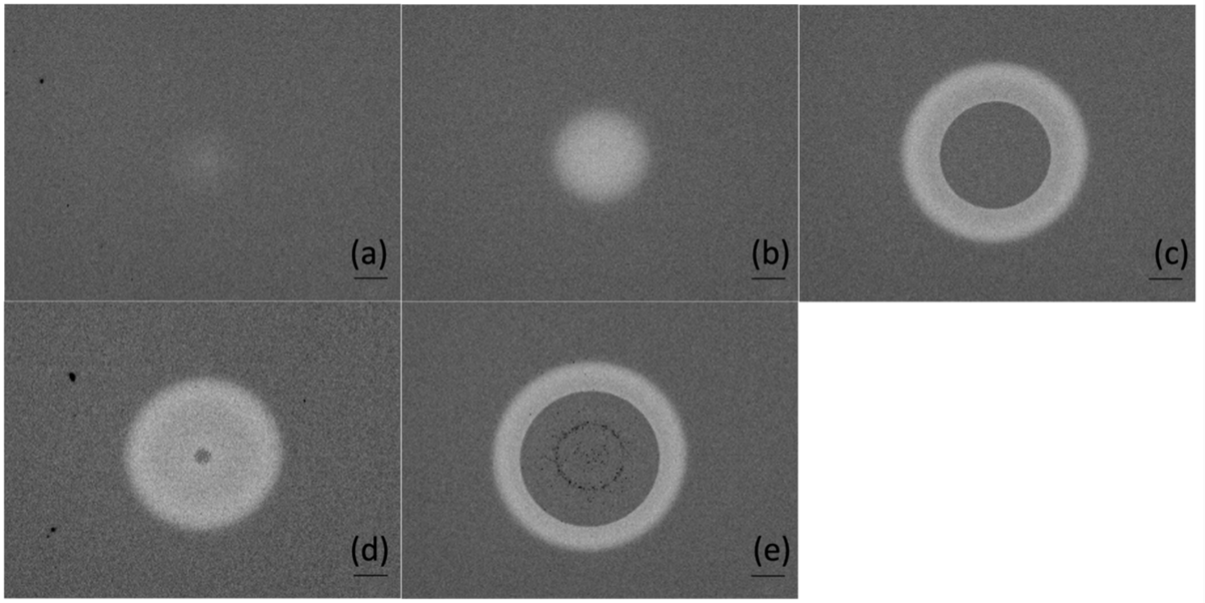


FIG. 1. Optical microscope image recorded in reflection of the surface of the 300 µm thick Si < 100 > wafer after single pulse exposure to a 800 nm, 15 fs laser pulse with a Gaussian intensity distribution, used for the beam waist determination and fluence calibration. The different images present the surface damage after a different fluence (a) 126 mJ/cm$^2$, (b) 138 mJ/cm$^2$, (c) 195 mJ/cm$^2$, (d) 240 mJ/cm$^2$ and (e) 300 mJ/cm$^2$. In (e) it is possible to observe 3 concentric rings, the bright outer ring corresponding to a thin amorphous layer formed upon melting and rapid quenching, an adjacent inner ring with the same a reflectivity as the unexposed material that corresponds to recrystallized material after melting and slower re-solidification and a central disk, delimited by a thin circle composed of micro-nanoparticles, which corresponds to the central region of highest fluence in which a thin surface layer has been ablated leaving behind re-crystallized material.

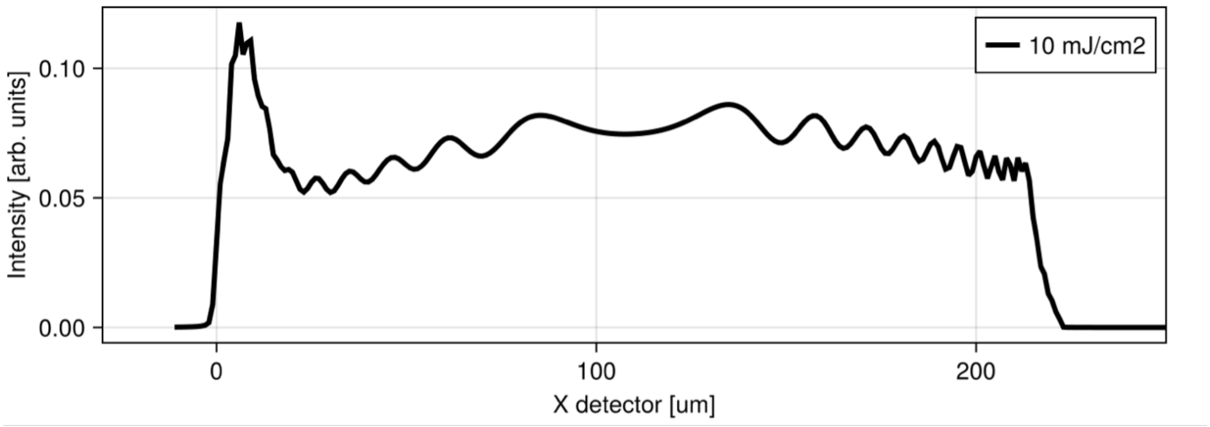


FIG. 2. Simulated profile of the diffraction signal using the Thomsen analytical model [1] at a delay of 900 ps, laser penetration length of 300 nm and a fluence of $10\,\mathrm{mJ/cm^2}$.

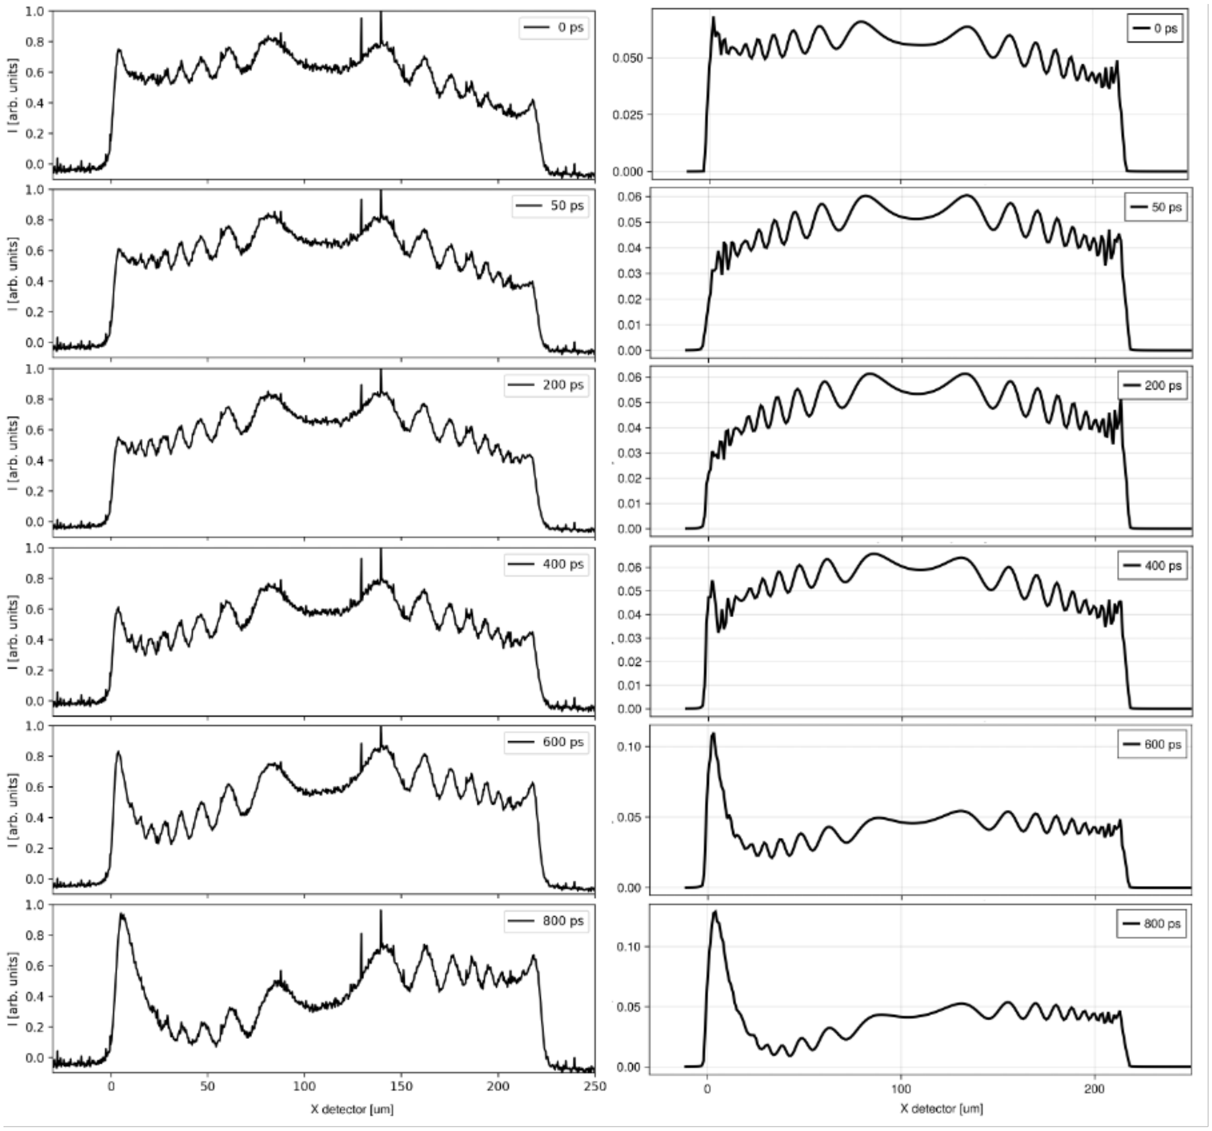


FIG. 3. (Left) Experimental depth profiles of the diffraction signal upon excitation at F = $52\,\mathrm{mJ/cm^2}$. Five different pump-probe delays between 0 and 800 ps are plotted. (Right) Corresponding simulated depth profiles using $F = 50\,\mathrm{mJ/cm^2}$ and a laser penetration depth d = 300 nm.
